# Supplementary material for: VulMatch: Binary-level Vulnerability Detection Through Signature
Source: arXiv:2308.00288 source file (2024-01-18)
Supplement: Supplementary file 1 [file appendix.tex]

\documentclass[lettersize,journal]{IEEEtran}
\usepackage{amsmath,amsfonts}
\usepackage{algorithmic}
\usepackage{algorithm}
\usepackage{array}
\usepackage{subcaption}
\usepackage{textcomp}
\usepackage{stfloats}
\usepackage{url}
\usepackage{verbatim}
\usepackage{graphicx}
\usepackage{cite}
\usepackage{xspace}
\usepackage{hyperref}
\usepackage{multirow}

\hyphenation{op-tical net-works semi-conduc-tor IEEE-Xplore}
% updated with editorial comments 8/9/2021

\begin{document}
\appendix
\input{07-appdx.tex}
\end{document}
